# Supplementary material for: Distributional Matrix Completion via Nearest Neighbors in the Wasserstein Space
Source: arXiv:2410.13112 source file (2026-12-01)
Supplement: Supplementary file 1 [file corr-appendix.tex]

% \begin{lemma}[\cref{assum:c_f} for \cref{cor:location-scale-bifactor}]\label{lemma:location-scale-bifactor-bound}
%     Here, we verify that \cref{assum:c_f} holds in the location-scale case in \cref{cor:location-scale-bifactor}. We have that $c_f = \frac{d}{\lambda_{\min}(\Sigma_{\mathrm{col}})}$ where $\Sigma_{\mathrm{col}} = \expect_{v \sim \mu_{\mathrm{col}}}*{vv^T}$.
% \end{lemma}
% \begin{proof}
%     By definition, we have
%     \begin{align*}
%         W_2^2(f(x,y),f(x',y))
%         &= \lVert \parenth{\sigma F_\mu^{-1} + \langle x,y \rangle} - \parenth{\sigma F_\mu^{-1} + \langle x',y \rangle} \rVert_{L^2(0,1)}^2 \\
%         &= {(\langle x,y \rangle - \langle x',y \rangle)}^2 \\
%         &= {(\langle x - x',y \rangle)}^2.
%     \end{align*}
%     Next, we have that
%     \begin{align*}
%         \expect_{v \sim \mu_{\mathrm{col}}}*{{(\langle x - x',v \rangle)}^2}
%         &= {(x - x')}^T \expect_{v \sim \mu_{\mathrm{col}}}*{vv^T} (x-x') \\
%         &\geq \lambda_{\min}(\Sigma_{\mathrm{col}}) \lVert x-x'\rVert^2.
%     \end{align*}
%     Finally, we have that 
%     \begin{align*}
%     W_2^2(f(x,y),f(x',y))
%     &= {(\langle x - x',y \rangle)}^2 \\
%         &\leq \lVert x-x'\rVert^2 \lVert y\rVert^2 \\
%         &\leq \frac{\lVert y\rVert^2}{\lambda_{\min}(\Sigma_{\mathrm{col}})}\expect_{v \sim \mu_{\mathrm{col}}}*{(\langle x - x',v \rangle)^2} \\
%         &\leq \frac{d}{\lambda_{\min}(\Sigma_{\mathrm{col}})}\expect_{v \sim \mu_{\mathrm{col}}}*{(\langle x - x',v \rangle)^2}. \\
%         &= \frac{d}{\lambda_{\min}(\Sigma_{\mathrm{col}})} \expect_{v \sim \mu_{\mathrm{col}}}*{W_2^2(f(x,v),f(x',v))}.
%     \end{align*}
% \end{proof}

% \begin{lemma}[\cref{assum:c_f} for \cref{cor:location-scale-ind}]\label{lemma:location-scale-ind-bound}
%     Here, we verify that \cref{assum:c_f} holds in the location-scale case in \cref{cor:location-scale-ind}. So, each row determines location and each column determines scale. Then, we have $c_f = 1$. If we reverse the roles of rows and columns where columns determine location and rows determine scale, then $c_f=1$ again.

%     In other words we have for any $x,x' \in \Hrow, y \in \Hcol$
%     \[
%     W_2^2(f(x,y),f(x',y)) = \expect_{v \sim \Hcol}*{W_2^2(f(x,v),f(x',v))}.
%     \]
% \end{lemma}
% \begin{proof}
%     In the first case, we have
%     \begin{align*}
%         W_2^2(f(x,y),f(x',y))
%         &= \left\lVert (yF^{-1} + x) - (yF^{-1} + x')\right\rVert_{L^2(0,1)}^2 \\
%         &= (x-x')^2.
%     \end{align*}
%     So, taking expectations over the columns (the second argument in $f$) does not change this calculation.
%     In the second case, we have
%     \begin{align*}
%         W_2^2(f(x,y),f(x',y))
%         &= \left\lVert (xF^{-1} + y) - (x'F^{-1} + y)\right\rVert_{L^2(0,1)}^2 \\
%         &= (x-x')^2 \left\lVert F^{-1}\right\rVert_{L^2(0,1)}^2.
%     \end{align*}
%     Again, taking expectations over the columns does not change this calculation.
% \end{proof}
